# Supplementary material for: Elucidating atmospheric brown carbon -- Supplanting chemical intuition with exhaustive enumeration and machine learning
Source: arXiv:2101.07301 ancillary file (2021-01-18)
Supplement: Supplementary file 1 [file SI_Atmospheric_Machine_Learning.pdf]

# Supporting Information: Elucidating atmospheric brown carbon – Supplanting chemical intuition with exhaustive enumeration and machine learning

Enrico Tapavicza,<sup>\*,†</sup> Guido Falk von Rudorff,<sup>‡</sup> David O. De Haan,<sup>¶</sup> Mario Contin,<sup>§</sup> Christian George,<sup>||</sup> Matthieu Riva,<sup>||</sup> and O. Anatole von Lilienfeld<sup>‡</sup>

<sup>†</sup>*Department of Chemistry and Biochemistry, California State University, Long Beach, 1250 Bellflower Boulevard, Long Beach, CA, 90840, USA*

<sup>‡</sup>*University of Vienna, Faculty of Physics, Kolingasse 14-16, AT-1090 Wien, Austria, and Institute of Physical Chemistry and National Center for Computational Design and Discovery of Novel Materials (MARVEL), Department of Chemistry, University of Basel, Klingelbergstrasse 80, CH-4056 Basel, Switzerland*

<sup>¶</sup>*Department of Chemistry and Biochemistry, University of San Diego, 5998 Alcala Park, San Diego, CA, 92110, USA*

<sup>§</sup>*Universidad de Buenos Aires, Facultad de Farmacia y Bioquímica, Departamento de Química Analítica y Fisicoquímica, Junín 956, Buenos Aires, C1113AAD, Argentina*

<sup>||</sup>*Université Lyon, Université Claude Bernard Lyon 1, CNRS, IRCELYON, 69626 Villeurbanne, France*

E-mail: enrico.tapavicza@csulb.edu

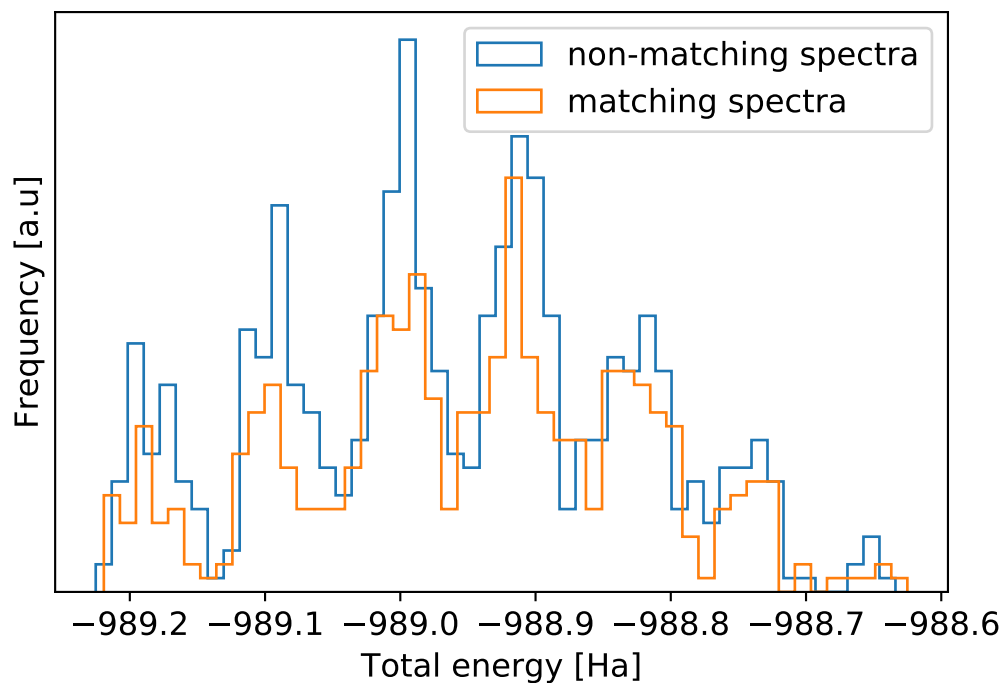

Figure 1: Histogram of total energies in the data set grouped into those molecules matching and not matching the experimental spectrum. For each group of molecules with the same property fingerprint, a subset of 2% of the molecules (at most 2000) have been calculated at RI-PBE0/def-SVP level.

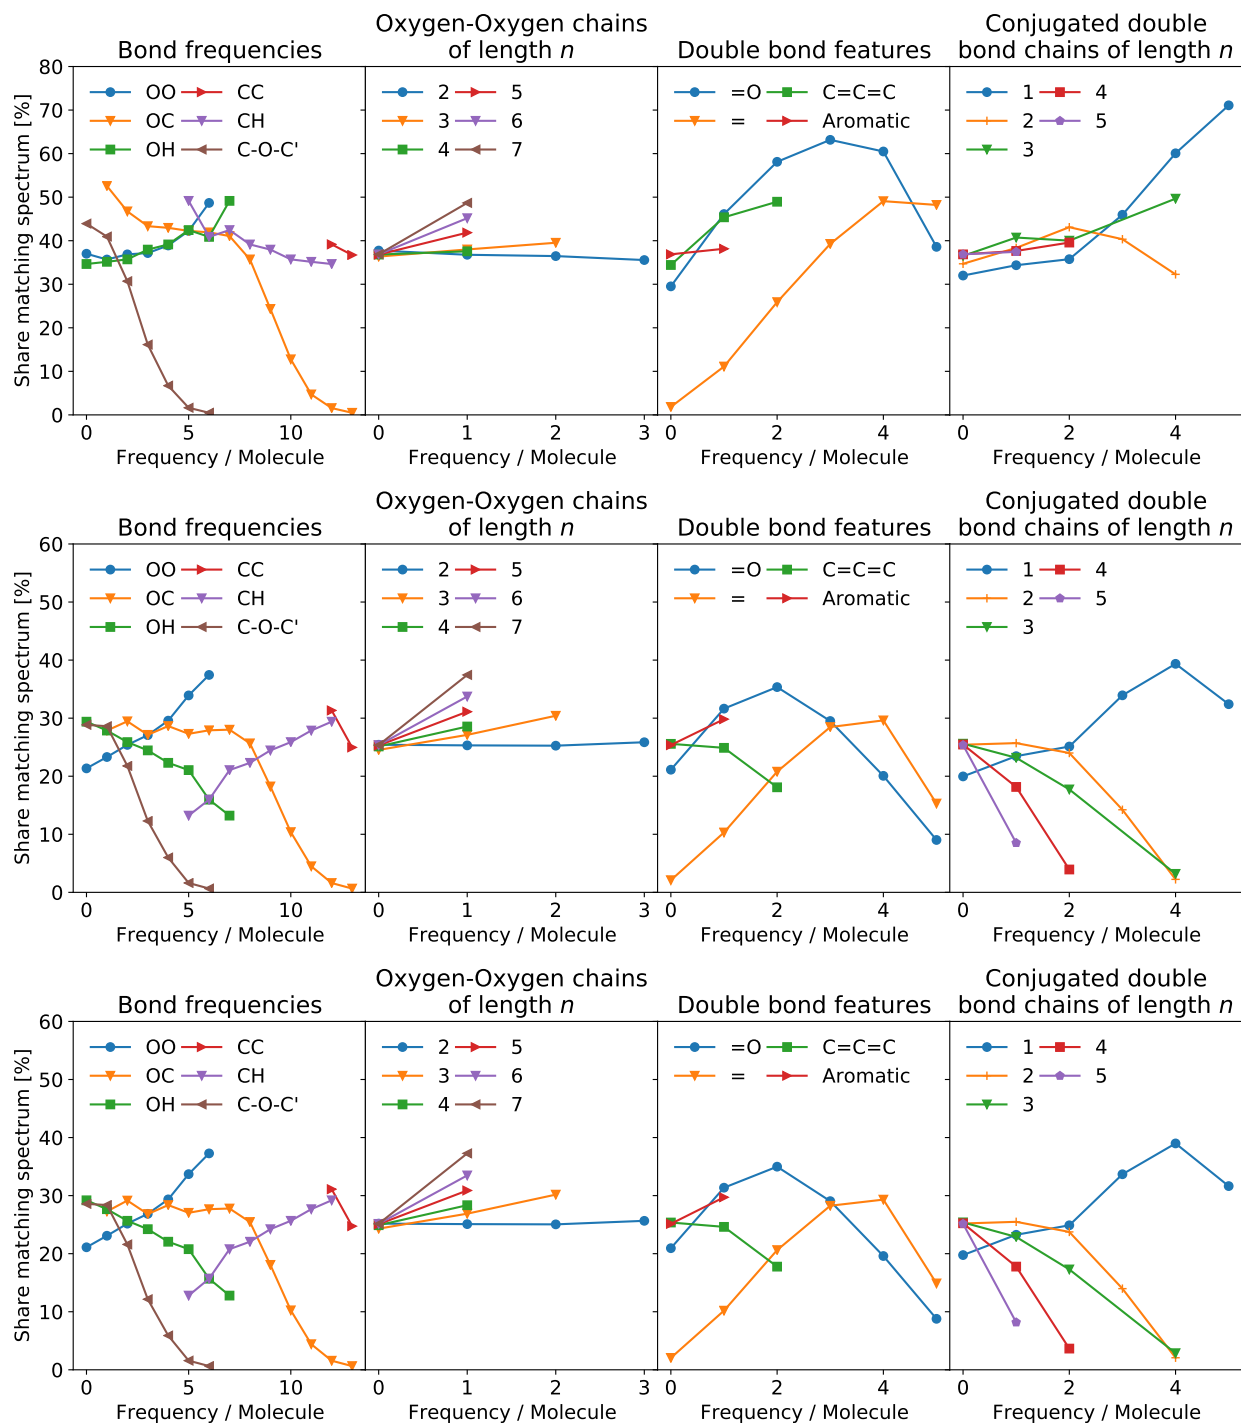

Figure 2: Share of all molecules of a given feature to be stable and compatible with the measured spectrum.

## 2 Molecule generation

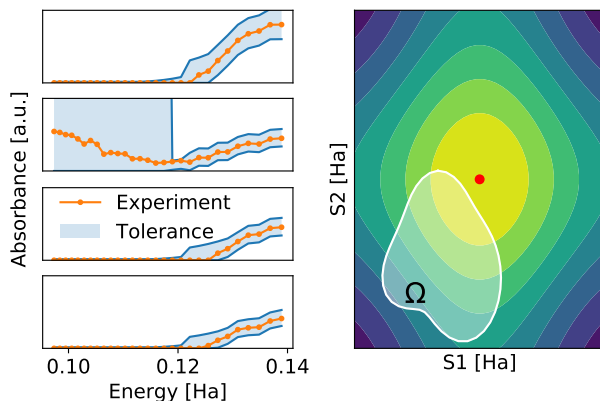

Figure 3: Left: The four different spectra of  $C_{12}O_7H_{12}$  isomers, obtained at different retention times from LCMS. Absorbance given in arbitrary units (a.u.). The shaded tolerance region defines the range within which the computational spectrum needs to fall to be treated as compatible. Right: Schematic representation to illustrate the matching probability. The red point represents the ML-predicted value in a two-dimensional parameter space.  $\Omega$  is the unknown parameter space within which the spectrum would be compatible with a given experimental one. The contour lines show the joint probability of a given parameter combination centered at the ML prediction. The not normalized probability of this ML prediction being compatible with the experimental spectrum is the integral over the joint probability within  $\Omega$ . This integral is approximated with the Monte-Carlo procedure described in the text.

3 We enumerate all potential molecular graphs by first listing all connected graphs with 9  
4 nodes. Here, each oxygen is one node and each aromatic ring is considered to be one. In the  
5 following, we refer to this case as reduced molecular graph. We filter this list to only include  
6 graphs with at most two nodes of degree six or less (i.e. at most two nodes may have up to  
7 six non-hydrogen bonds), while all other nodes may be at most of degree two (i.e. have two  
8 bonds). For this, we used nauty 27rc3.<sup>1</sup> The graph theory analog for the element of an atom  
9 is the color of a node. We then build a list of all possible colorings of the previously obtained  
10 graphs. For each graph, we enumerate all combinatorically possible bonded hydrogen counts  
11 for each site, which leaves 21.513 graphs. Note that at this stage, the enumeration does  
12 not contain molecular graphs yet, since the  $C_6$  rings are treated as one node and no valence  
13 rules are followed. In this first step, no duplicates can occur in the list of reduced molecular

graphs.

In the second step, we take all reduced molecular graphs and reconstruct all possible hydrogen saturations. While limits on the hydrogen count per node are already given in the reduced molecular graph, one node can be a full  $C_6$  ring. This step enumerates all possible positions for this number of hydrogens over the six positions of the ring. Effectively, this requires finding all integer partitions of the total number of bonds formed for this ring (including the other ring and potentially all oxygens) under the condition that bond valence consideration are satisfied: each hydrogen must have exactly one bond, each oxygen has exactly two bonds (or one double-bond), and each carbon has four single-bond equivalents. Since the integer partitions might yield duplicates, we use the graph isomorphism check `vf22` to sieve out duplicates. Since isomorphism checks are computationally demanding, we performed a pre-screening exploiting that the spectrum of the adjacency matrix is an incomplete graph invariant, so exact isomorphism checks were only needed for those of identical spectrum. This step yielded 263.917.411  $C_{12}O_7H_{12}$  molecules in total. All generated molecules contains exactly seven double bond equivalents, that is either close rings or double bonds. Of those seven double bond equivalents, at least two must be closed rings ( $C_6$ -rings).

For each molecule, we used `openbabel3,4` to generate an initial guess of the 3D structure using their C++ interface. The initial guess was subsequently relaxed using `MMFF945` as implemented in `openbabel` using steepest descent for 500 steps to remove bad contacts from the initial guess of the structure. The resulting structure was further minimized to convergence using the density functional tight binding variant `GFN2-xTB6` as implemented in `xtb 6.2.2`. A molecule was considered stable if a) the minimization converged and b) the molecular graph as detected from Wiberg bond orders<sup>7</sup> did not differ at the end of the minimization from generated input molecular graph. After this step, 123.354.268 stable  $C_{12}O_7H_{12}$  molecules were left.

## Machine learning

To determine optimal hyperparameters, i.e. kernel widths  $\sigma$  and regularizer  $\lambda$ , ML calculations with training set sizes 100, 1000, 3000, 5000, and 9000 were carried out; a 5-fold cross-validation was used, where remaining molecules were used as out-of-sample validation sets. The determined optimal kernel widths were  $\sigma = 65.536$  for the learning of the energies and  $\sigma = 0.128$  for oscillator strengths; a regularizer of  $\lambda = 10^{-7}$  was found to be optimal in both cases. These parameters were used for the predictions of the remaining molecules.

## Monte-Carlo algorithm to establish matching of experimental spectra

Wavelength-dependent molar extinction coefficients of  $\text{C}_{12}\text{O}_7\text{H}_{12}$  were estimated from absorbance spectra recorded (Fig. 3) at four different retention times of sodium adducts of  $\text{C}_{12}\text{O}_7\text{H}_{12}$  using the Beer-Lambert equation.

Surrogate standards were used to quantify electrospray ionization efficiencies and therefore concentration, and the photodiode array pathlength was 1 cm. Since ionization efficiencies vary significantly between compounds, the use of surrogate standards introduces an order-of-magnitude uncertainty.

Since each energy and oscillator strength is subject to uncertainties from the machine learning prediction, we employ a Monte Carlo scheme to obtain the likelihood of the molecule having a spectrum that is compatible with the experimental spectrum. This is done by drawing 10.000 random excitation energies and oscillator strengths from a joint probability distribution centered around the machine learning predictions with the uncertainties from the test set used in machine learning. For each such drawn set of parameters, the spectrum has been calculated, employing a typical full-width-at-half maximum of 0.3 eV,<sup>8,9</sup> and tested whether it is within the corridor in Figure 3. The fraction of spectra compatible with the experimental one is the probability that the spectrum of this molecule is compatible with

the experimental one given the uncertainties of the machine learning predictions. In the limit of no uncertainties, this would leave exactly the matching molecules with a non-zero probability.

Assuming that our set of molecules also contains the molecule that gave rise to the experimental spectrum, this one molecule would have the largest overlap with the volume in parameter space that is compatible with the spectrum. Since no molecule has a probability close to one, our uncertainties (which are assumed to be identical for all molecules) need to be wider than this parameter space. We use this fact to derive a minimum threshold for the Monte Carlo probability: While we do not know the full parameter space that is compatible with the experimental spectrum, we know that the largest likelihood of all molecules is the integral over that space convolved with the given probability distribution centered over that space. Now if each of the six parameters were drawn exactly one standard deviation away from the center of the probability function, the product of these probabilities would be  $\exp(-3) \simeq 1/20$  of the likelihood at the center of all six normal distributions. Therefore, our threshold is  $\exp(-3)$  of the largest likelihood obtained in our list of molecules. In total, 54.797.670 molecules have a likelihood above that threshold and therefore are considered to be compatible with the experimental spectrum.

## **C<sub>12</sub>H<sub>12</sub>O<sub>7</sub> structure proposed by Laskin et al.**

Table 1: Excitation energies of the structure found by Laskin et al.,<sup>10</sup> computed by ADC(2)/COSMO.

| Excitation energy (au) | oscillator strength (au) |
|------------------------|--------------------------|
| 0.11673793986005E+00   | 0.88706001377993E-01     |
| 0.13710157179088E+00   | 0.10327306454072E-03     |
| 0.14767512555885E+00   | 0.75348944434187E-01     |

Table 2: GFN-XTB optimized coordinates of the structure porposed by Laskin et al.<sup>10</sup>

|   |            |            |            |
|---|------------|------------|------------|
| O | -4.7520756 | 2.6163567  | -0.3233092 |
| O | -5.7165298 | 0.3033973  | 1.2685487  |
| O | -2.1447097 | 2.7139311  | -0.9847708 |
| O | -0.3799121 | 0.7840369  | -0.0923865 |
| O | 0.8357602  | -2.3670248 | 0.6235432  |
| O | 0.5964942  | -3.3748992 | 3.0278621  |
| O | -1.1510866 | -3.5129848 | 4.3687891  |
| C | -3.9614721 | 1.5965041  | 0.1097260  |
| C | -2.6050057 | 1.6348832  | -0.2230492 |
| C | -4.4368086 | 0.5191445  | 0.8730105  |
| C | -1.7032247 | 0.6635363  | 0.1974323  |
| C | -2.1759187 | -0.4122345 | 0.9561946  |
| C | -3.5279396 | -0.4573902 | 1.2692086  |
| C | -1.2283545 | -1.4394733 | 1.4235205  |
| C | -0.2390121 | -1.8524841 | 0.4146969  |
| C | -1.3347564 | -1.9240510 | 2.6793222  |
| C | -0.6124049 | -3.0094595 | 3.4138346  |
| C | -6.7064369 | 1.2859665  | 1.0453324  |
| C | -2.1078389 | 2.4485213  | -2.3816930 |
| H | -3.9195385 | -1.2859164 | 1.8368052  |
| H | -4.1647116 | 3.2832079  | -0.7145066 |
| H | -0.2327707 | 1.6698580  | -0.4565927 |
| H | -7.6120480 | 0.8838209  | 1.4969877  |
| H | -6.8738945 | 1.4572247  | -0.0199502 |
| H | -6.4481590 | 2.2316336  | 1.5267918  |
| H | -1.4430086 | 1.6115489  | -2.6138398 |
| H | -1.7291544 | 3.3555536  | -2.8489759 |
| H | -3.1049385 | 2.2215392  | -2.7702723 |
| H | 0.8894459  | -2.9521175 | 2.1813959  |
| H | -0.5630925 | -1.6559541 | -0.6193680 |
| H | -2.1416070 | -1.5335854 | 3.2885017  |

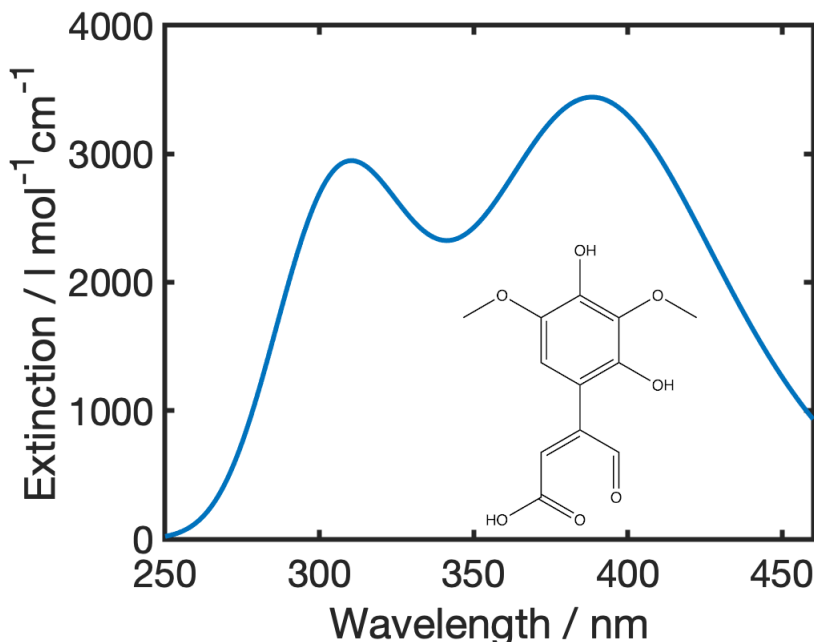

Figure 4: Absorption spectrum for the  $C_{12}H_{12}O_7$  structure (shown) proposed by Laskin et al. The spectrum was simulated based on ADC2/COSMO excitation energies and oscillator strengths (Table 1), using a Gaussian line shape with a full width at half maximum of 0.3 eV.

## References

- (1) McKay, B. D.; Piperno, A. Practical graph isomorphism, {II}. *Journal of Symbolic Computation* **2014**, *60*, 94 – 112.
- (2) Cordella, L. P.; Foggia, P.; Sansone, C.; Vento, M. A (sub)graph isomorphism algorithm for matching large graphs. *IEEE Transactions on Pattern Analysis and Machine Intelligence* **2004**, *26*, 1367–1372.
- (3) O’Boyle, N. M.; Banck, M.; James, C. A.; Morley, C.; Vandermeersch, T.; Hutchison, G. R. Open Babel: An open chemical toolbox. *Journal of cheminformatics* **2011**, *3*, 33.
- (4) Open Babel version 2.4.0. [openbabel.org](http://openbabel.org), accessed 2020-03-01.
- (5) Halgren, T. A. Merck molecular force field. I. Basis, form, scope, parameterization, and performance of MMFF94. *Journal of computational chemistry* **1996**, *17*, 490–519.

- (6) Bannwarth, C.; Ehlert, S.; Grimme, S. GFN2-xTB—An accurate and broadly parametrized self-consistent tight-binding quantum chemical method with multipole electrostatics and density-dependent dispersion contributions. *J. Chem. Theory Comput.* **2019**, 1652–1671.
- (7) Wiberg, K. B. Application of the pople-santry-segal CNDO method to the cyclopropylcarbinyl and cyclobutyl cation and to bicyclobutane. *Tetrahedron* **1968**, 24, 1083–1096.
- (8) Schalk, O.; Geng, T.; Thompson, T.; Baluyot, N.; Thomas, R. D.; Tapavicza, E.; Hansson, T. Cyclohexadiene Revisited: A Time-Resolved Photoelectron Spectroscopy and ab Initio Study. *J. Phys. Chem. A* **2016**, 120, 2320.
- (9) Epstein, S. A.; Tapavicza, E.; Furche, F.; Nizkorodov, S. A. Direct photolysis of carbonyl compounds dissolved in cloud and fog droplets. *Atmos. Chem. Phys.* **2013**, 13, 9461–9477.
- (10) Yu, L.; Smith, J.; Laskin, A.; Anastasio, C.; Laskin, J.; Zhang, Q. Chemical characterization of SOA formed from aqueous-phase reactions of phenols with the triplet excited state of carbonyl and hydroxyl radical. *Atmos. Chem. Phys.* **2014**, 14, 13801–13816.
